# Supplementary material for: Ultrafast X-ray Spectroscopy of Intersystem Crossing in Hexafluoroacetylacetone: Chromophore Photophysics and Spectral Changes in the Face of Electron Withdrawing Groups
Source: arXiv:2209.13149 ancillary file (2022-12-13)
Supplement: Supplementary file 1 [file HfAcAc_SI.pdf]

# Supporting Information

# Influence of Electron Withdrawing Groups on Ultrafast Intersystem Crossing by Transient X-ray Absorption Spectroscopy at the Carbon K-Edge

**Eric A. Haugen,†‡ Diptarka Hait,†‡ Valeriu Scutelnic,†‡ Tian Xue,†‡ Martin Head-Gordon,†‡ and Stephen R. Leone†‡¶**

**Department of Chemistry, University of California, Berkeley, CA 94720, USA†**

**Chemical Sciences Division, Lawrence Berkeley National Laboratory, Berkeley, CA 94720,USA ‡**

**Department of Physics, University of California, Berkeley, CA 94720, USA ¶**

## S1. Expanded Experimental Methods:

A high harmonic source was used to generate broadband soft X-ray pulses extending to the carbon K-edge (160-350 eV, sub-60 fs), which serves as the probe. Full details of the experimental apparatus and a schematic of the layout are provided elsewhere.[1] Briefly, the output of an optical parametric amplifier (HE-TOPAS, Light Conversion, 1180-2600 nm) at 1470 nm (2.5-3.0 mJ/pulse) is focused into a differentially pumped semi-infinite gas-cell filled with 1300-1500 Torr of helium to generate the high harmonics. The residual infrared beam is filtered by a 100 nm thick Al filter and the transmitted X-rays are then imaged by a toroidal mirror onto a sample cell at a measured $1/e^2$ beam-waist of 65 ± 2μm. Further filtering of the X-rays is conducted using two 50 nm thick Ti filters; these act as a seal between the sample chamber and adjacent chambers, negating the risk of gas contamination of X-ray optics and blocking residual pump beam light.

The OPA is pumped by a 90% split-off of the 800 nm output (12 W, 1 kHz, sub-45 fs pulse duration of a commercial Ti:Sapphire laser (Spit- fire Ace, Spectra Physics). The second split-off portion of the output is attenuated to 800 $\mu$J/pulse by a 70:30 beam splitter and used to generate the third harmonic (266 nm, 120 μJ/pulse, sub-70 fs pulse width). The ω + 2ω mixing crystal is detuned to restrict the pump pulse energies to below 40 μJ/pulse. About 60% throughput of these pulse energies is measured through the sample cell. A D-mirror is used to provide a shallow angle (1°) between the pump and probe beam for spatial overlap between the

two beams. The UV beam is routed into the sample cell via a temporal delay stage (1 fs step-size) and the small angle of 1° results in minimal temporal broadening from group velocity mismatch of the angles. The transmitted X-rays are dispersed using a variable line spaced Hitachi grating (001-0660) with a nominal 1200 lines/mm at an 87° angle of incidence to disperse the X-rays onto a translatable X-ray camera (Princeton Instruments, PIXIS:XO 400B). The energy resolution of the spectrometer is 320 meV at 244 eV (Figure S1) and the temporal instrument response function (IRF) is 80 fs, as measured in previously conducted experiments on the instrument.[2]

The ambient vapors of HfAcAc (Sigma Aldrich, cooled to – 5 °C) are made to flow through a sample cell with a path length of 8 mm, with the pump and probe beams transmitted through 300 μm holes in the sides of the gas cell. The sample cell is heated to 60 °C to reduce clogging. The static X-ray absorption spectra are acquired by measuring the X-rays transmitted through the sample cell, both in the presence ($I_{in}$) and absence ($I_{out}$) of the sample vapors to obtain the absorbance, $A = -\log_{10}(I_{in}/I_{out})$. Typically, the spectra are measured by referencing 64 averaged CCD images (1000 laser pulses per image) corresponding to each of $I_{in}$ and $I_{out}$. Three of these spectra were averaged for improved signal-to-noise ratio. Standard scans would include timepoints out to 10ps while additional timepoints at longer delays were also taken with fewer averages. The energy calibration of the spectrometer is performed by comparison with the reported $2p^{-1}4s$ and $2p^{-1}nd$ resonances of Argon[3] (Figure S1) as well as the C 1s π* resonance of the allyl radical[4], produced by the 266 nm photodissociation of allyl iodide.

## S2. Experimental energy resolution probed at the Ar $L_{2,3}$ edge

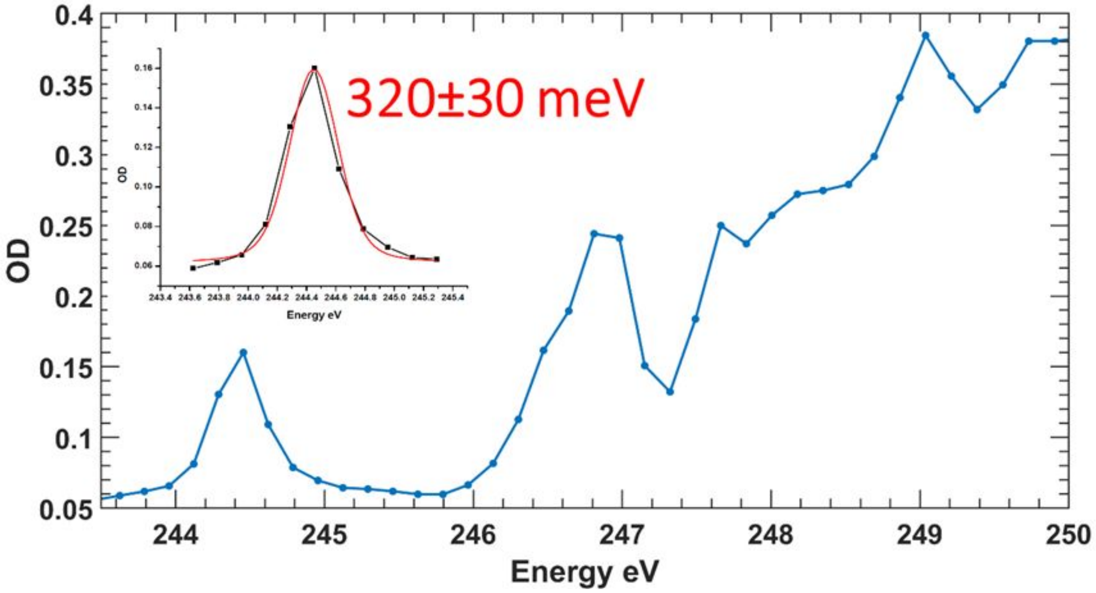


**Figure S1.** Near-edge X-ray absorption fine structure (NEXAFS) spectrum of argon shows the atomic core-to-Rydberg state resonances that are used to calibrate the spectrometer. Inset shows the fitting of the $2p_{3/2}$→4s resonance to a Voigt line shape with a fixed Lorentzian width of 114 meV[3] (core-hole lifetime broadening) to extract the Gaussian width, which provides the spectrometer resolution of 320±30meV.

## S3. Power dependence of X-ray signal

The sample was irradiated with a 266 nm pulse energy ranging from 5-25 □J. The change in X-ray absorption signal corresponding to this power dependence is shown in Figure S2. It might be expected that multiphoton excitation could result in the production of higher excited states ( such as excitations into the Rydberg orbitals) or ionization of the molecule. From the linear power dependences of the X-ray absorption features, it is expected that these potential nonlinear outcomes will constitute a small fraction of the excited species. No such species are evident in the data at the higher power densities. An excitation percentage of 20% was determined in the pump-probe interaction volume under the experimental conditions. It was determined that a 20% excitation was sufficient for removing discontinuities and negative signal originating from the ground state bleach in the excited state spectra. All absorption measurements were performed in the linear regime. Peak 8 corresponds to a high energy excitation arising from the $CF_3$ carbons, which is shown in more detail in Figures S3 and S4.

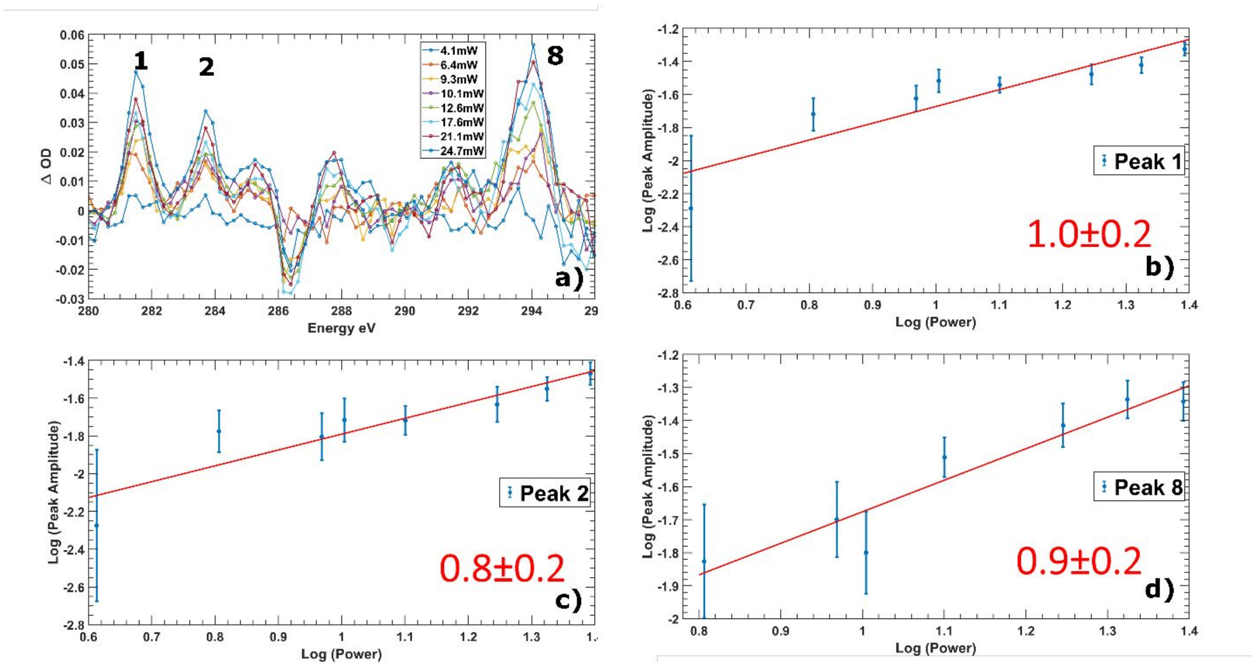


**Figure S2.** Power dependence measurements on HfAcAc from 4.1-24.7 □J excitation at 5 ps delay. (a) displays each spectrum at its respective pump power. (b) & (c) correspond to the 1s → □* transition for the $T_1$ state, which are labeled peaks 1 & 2, respectively, in the main text. (d) corresponds to an intense high energy feature at 294 eV driven by excitations from the $CF_3$ carbons. The power corresponding to 4.1 □J excitation is excluded in the fit given the low signal-to-noise ratio observed, producing an anomalously low intensity excitation. The signals arising from the high energy excitations are shown in more detail in Figure S3 & S4.

The approximately unity linear fits demonstrate that the dynamics reported in the main manuscript arise from a single 266 nm photon excitation. It should be noted that the ultraviolet absorption cross section of hexafluoroacetylacetone (HfAcAc) is very high, thus lower power densities can be used, which may help ensure one-photon excitation. The production of ionized HfAcAc is deemed as unlikely due to the high ionization potential of HfAcAc (10.72 eV),[5] necessitating a three photon excitation to produce ions. Likewise, ionization of HfAcAc would result in a singly occupied molecular orbital, likely originating from the nonbonding oxygen p orbital of the C=O. Despite being located on the oxygen, it is expected that there would be a weak signal at the carbon K edge, as was seen in peaks A and B of the $S_1$ state, shown in Figure 4 of the main text. This signal would appear on the timescale of the instrument response function and would likely be long-lived and of constant intensity corresponding to a stable cation.

**S4. High Energy Features displaying transitions from the $CF_3$ carbons**

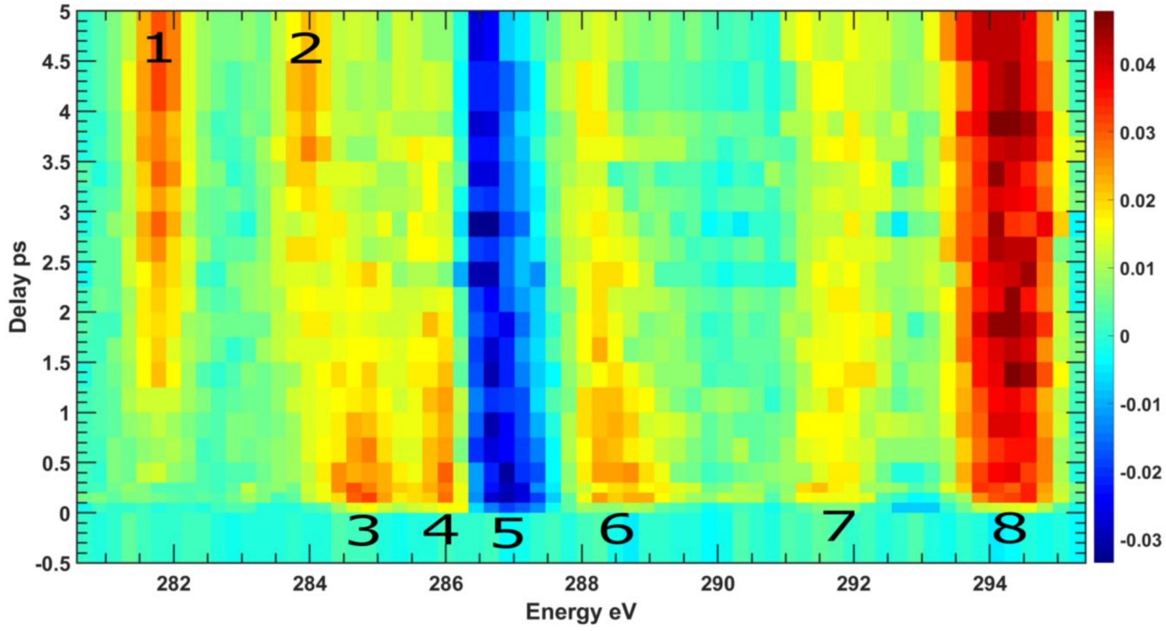


**Figure S3.** Experimentally measured, transient spectrum versus time of HfAcAc following excitation with 266 nm pump pulse for the full energy range.

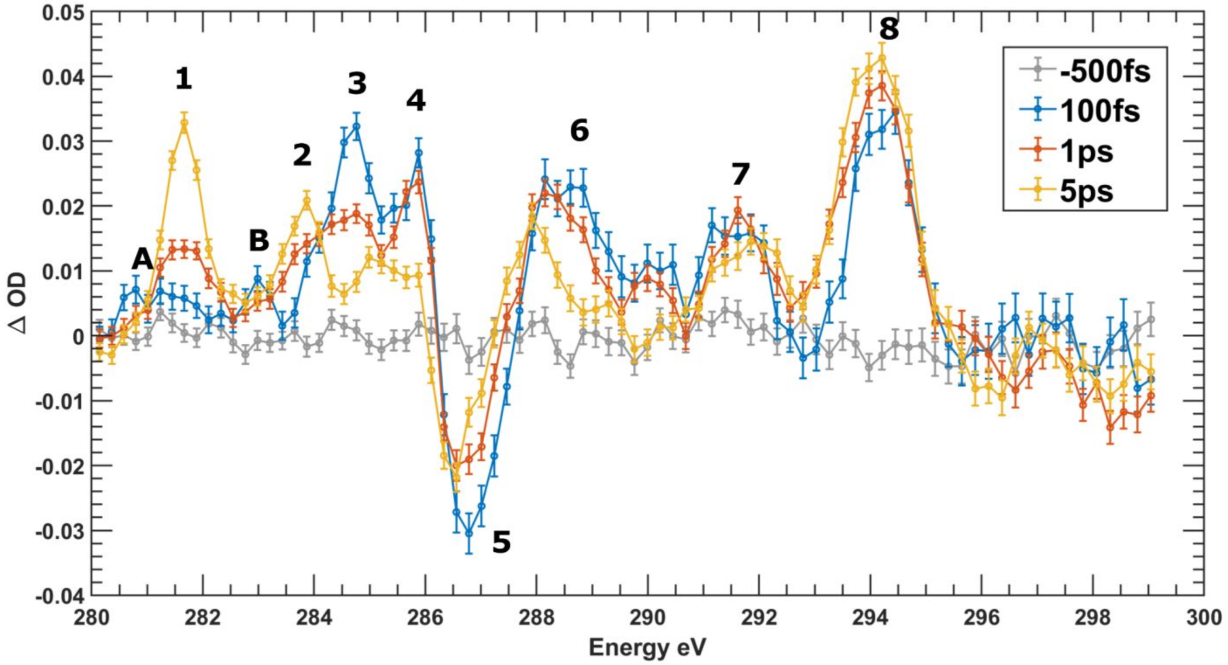


**Figure S4.** Full energy range displaying ΔOD at 100 fs, 1 ps, and 5 ps. Highlighting the shift from the singlet $S_1$ state to the triplet $T_1$ state. Peaks 1-8 correspond to the transitions observed in Figure S3, meanwhile transitions A and B correspond to weak 1s → n (singly occupied oxygen 2p lone-pair) transitions consistent with the $S_1$ state.

## S5. Long time dynamics

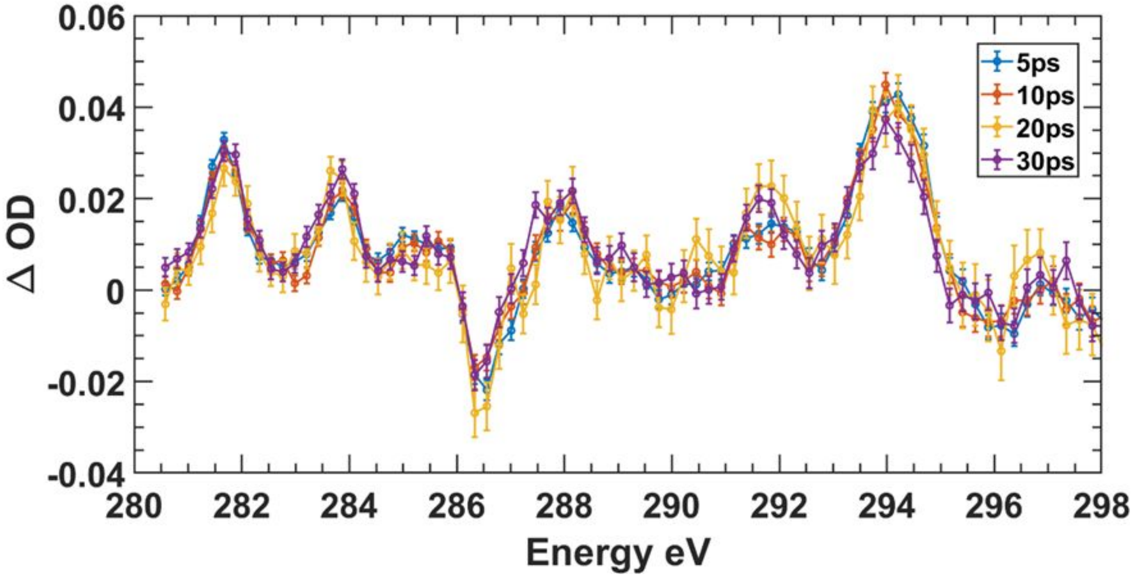


**Figure S5.** Long-time dynamics of HfAcAc; no distinguishable features above the signal-to-noise ratio are present at delays longer than 5 ps. It is determined that the triplet state is long-lived and does not readily relax down to the ground state nor dissociate into photoproducts with distinct spectral signatures in the timescales probed in this experiment.

## S6. Additional calculated electronic states and photoproducts

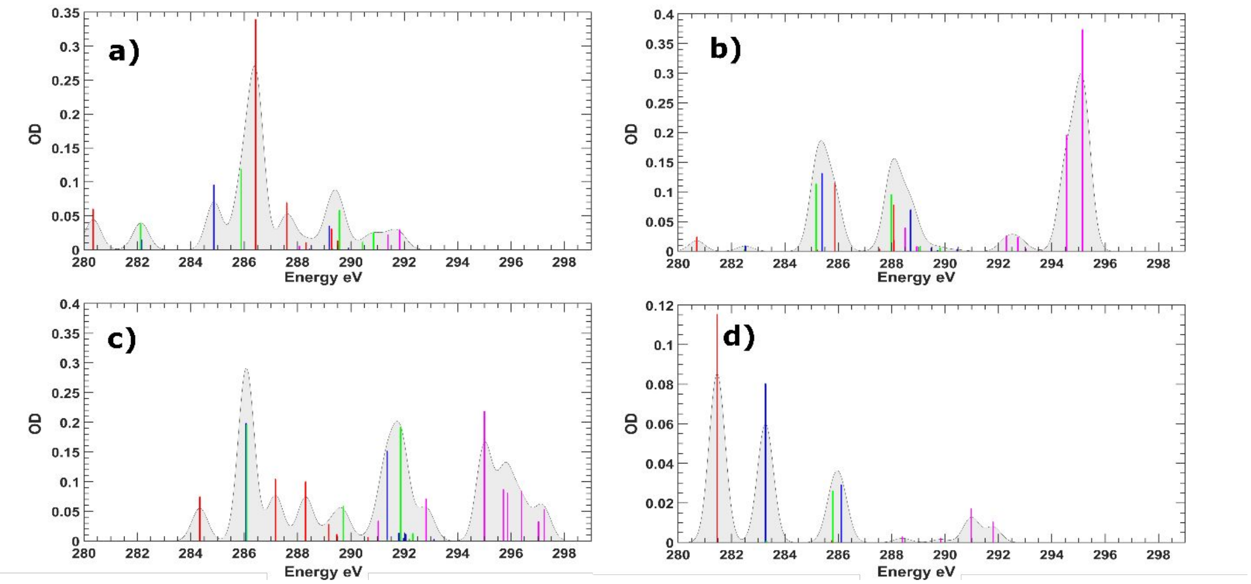


**Figure S6.** OO-DFT C K-edge calculations for low energy absorption features of the $S_2/S_1$ states of HfAcAc and possible $S_0/T_1$ pentafluoromethyl-3-furanone product. (a) corresponds to the $S_2$ electronic state at the optimized $S_0$ geometry (i.e. in the Franck-Condon region). (b) corresponds to the $S_1$ electronic state at the optimized $S_0$ geometry. (c) corresponds to the $S_0$ state of the possible pentafluoromethyl-3-furanone photoproduct at its optimized geometry. (d) corresponds to the pentafluoromethyl-3-furanone in the $T_1$ state at its optimized geometry.

It can be seen in Figure S6(a) that the $S_2$ excited state possesses lower energy transitions corresponding to the 1s→π transition originating at 280.3 eV for the $C_3$ carbon. Calculations corresponding to the Franck Condon (FC) region of excitation were performed in this case, due to the expected short lifetime of the $S_2$ state. Only minimal calculations are performed on the terminal $CF_3$ carbons due to the large number of overlapping transitions in this region of the spectrum, all of which are at higher energy. In Figure S6(b) the $S_1$ electronic state is calculated at the ground state geometry. Here it is observed that the splitting at short delays in the experimental spectrum at 284.6 and 286.1 eV is not present in the FC geometry spectra. This contrasts with Figures 5(a) and 5(b) in the main text where a clear splitting is observed at the $S_{1min}$ geometry and the $S_2/S_1$ minimum energy conical intersection geometry. This indicates that a considerable change in geometry from the FC region occurs prior to the detection of the $S_1$ excited state. Figure S6(c) corresponds to the simulated spectrum of pentafluoromethyl-3-furanone in the $S_0$ state. The low energy features match quite closely with the ground state and only predict significant differences for the $CF_3$ carbons where the peaks are observed to be redshifted. In Figure S6(d) the 1s→$\pi/\pi^*$ for the $T_1$ furanone are observed. Calculations to the low energy $\pi$ and $\pi^*$ states provide insights into the expected experimental signal present in the low energy region of the XAS spectrum. This spectral region has good signal-to-noise, given the

absence of ground state absorption, allowing only signals originating from the excited state to be observed. It may also be seen that the lowest energy transitions from the $T_1$ furanone is similar to the planar $T_1$ state of HfAcAc in Figure 5(d) of the main paper.

## S7. Short time scans

The $S_2$ state is not clearly observed in the experimental data (Figure S7.) at short time delays above the experimental noise. In AcAc it has been estimated that the lifetime of this $S_2$ state is on the order of 10-50 fs, shorter than the resolution of this experiment.[6,7] Features prior to time zero may be seen, due to the long pulse duration of the 266 nm light. At this time only a small fraction of the molecules are excited, resulting in a weak transient signal when probed with X-rays.

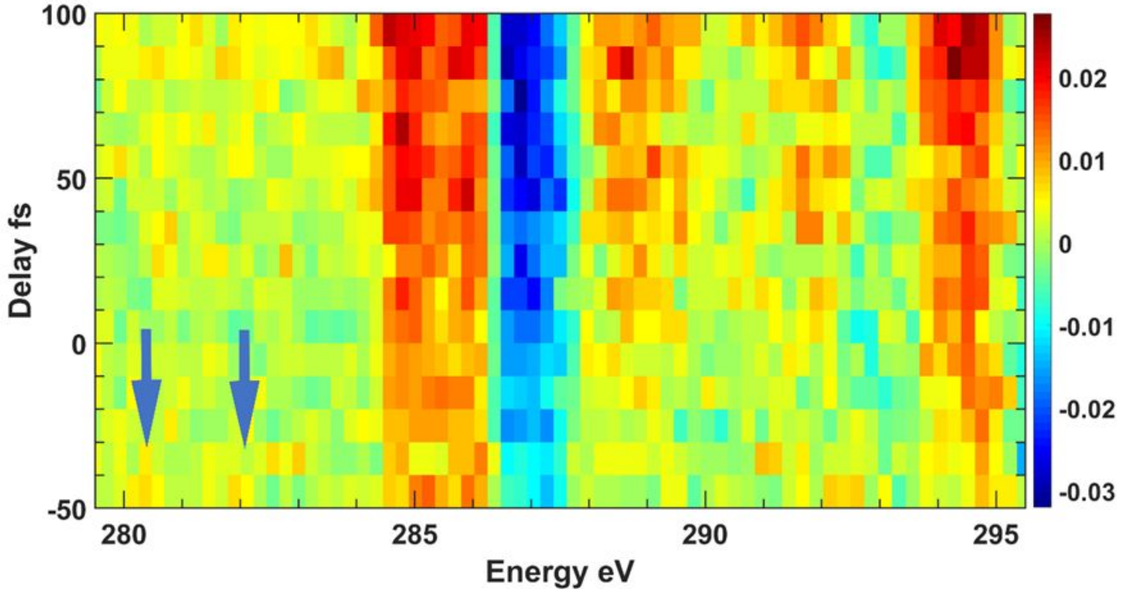


**Figure S7.** Contour Map of short delays, with a 10 fs step size, arrows are drawn to illustrate the energies of the calculated C 1s→π orbital of the $S_2$ state, as observed in Figure S6(a). This transition is located in the low energy region around 280 eV; here no significant signal from the ground state of HfAcAc allowing for the background free observation of any excited states in this energy region.

## S8. Rotational Isomers of the Triplet State

### Rotational isomers present in the $T_1$ state

Hexafluoroacetylacetone can potentially exist as eight rotationally distinct isomers (rotamers), as shown in Figure S8. Their nomenclature consists of three letters corresponding to a cis (C) or trans (T) configuration about each of the $C_2$-$C_3$, $C_3$=$C_4$ and $C_4$-OH bonds. The CCC form is the global minimum in the ground state, but the intramolecular hydrogen bond can potentially break upon excitation with 266 nm light and lead to other configurations. The TCC rotamer in particular has been predicted to be a possible precursor to the primary photoproduct of pentafluoromethyl-3-furanone.[8]

All eight rotamers can be obtained as local minima after geometry optimization in the $S_0$ state. Rotation about the $C_3$=$C_4$ bond however becomes possible in the $T_1$ state, and pairs of rotamers can thus collapse onto a single, twisted local minimum structure (for example, using $S_0$ optimized TCT and TTT initial geometries for the $T_1$ state optimization lead to the same minimum). Overall, the range of rotamer minimum energies in the $T_1$ state is computed to be 2 kcal/mol (vs 16.5 kcal/mol in the $S_0$ state), which is sufficiently small for interconversion to occur between rotamers, utilizing the energy gained from electronic relaxation from the $S_2$ state.

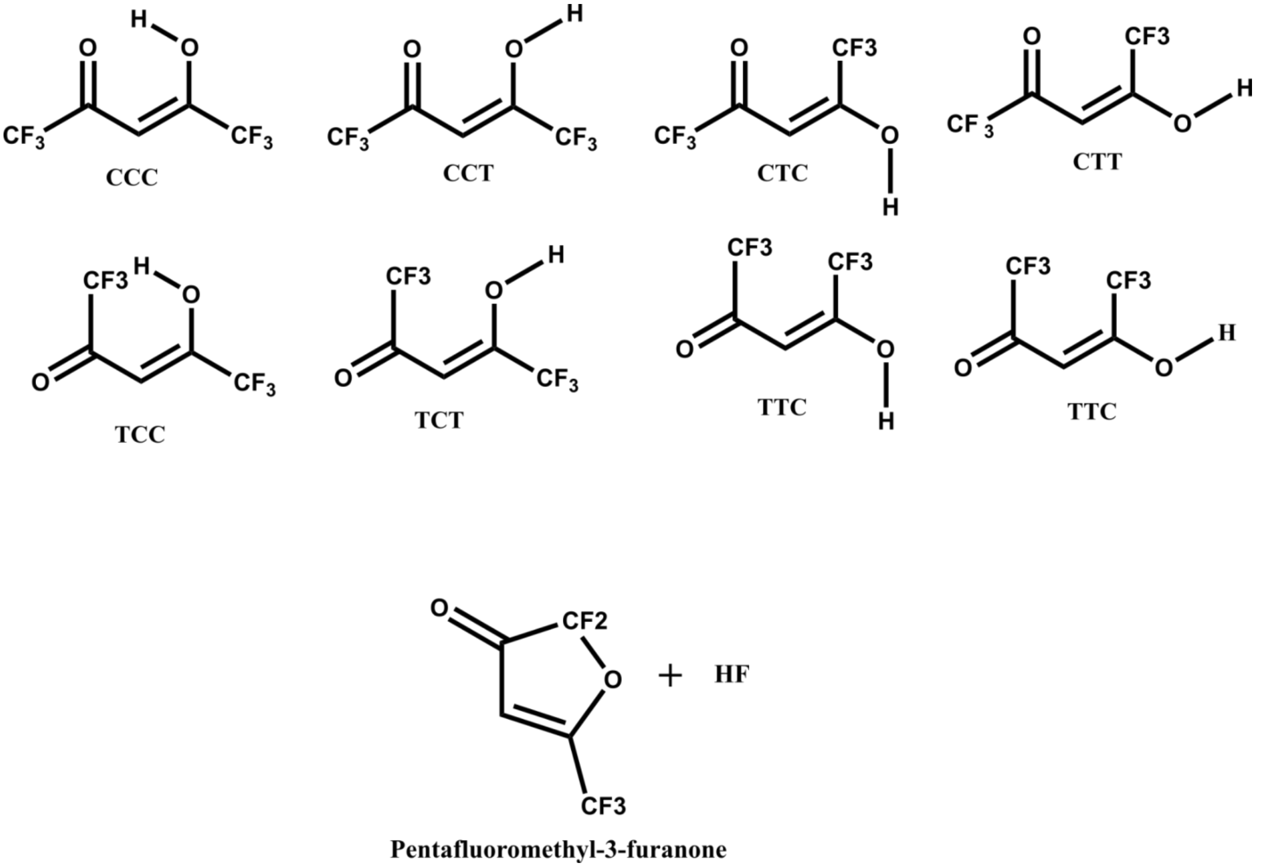


**Figure S8.** Various possible rotational isomers present in the $T_1$ state in addition to the Pentafluoromethyl-3-furanone product.

**Calculated Spectra for unique rotational isomers in the $T_1$ state**

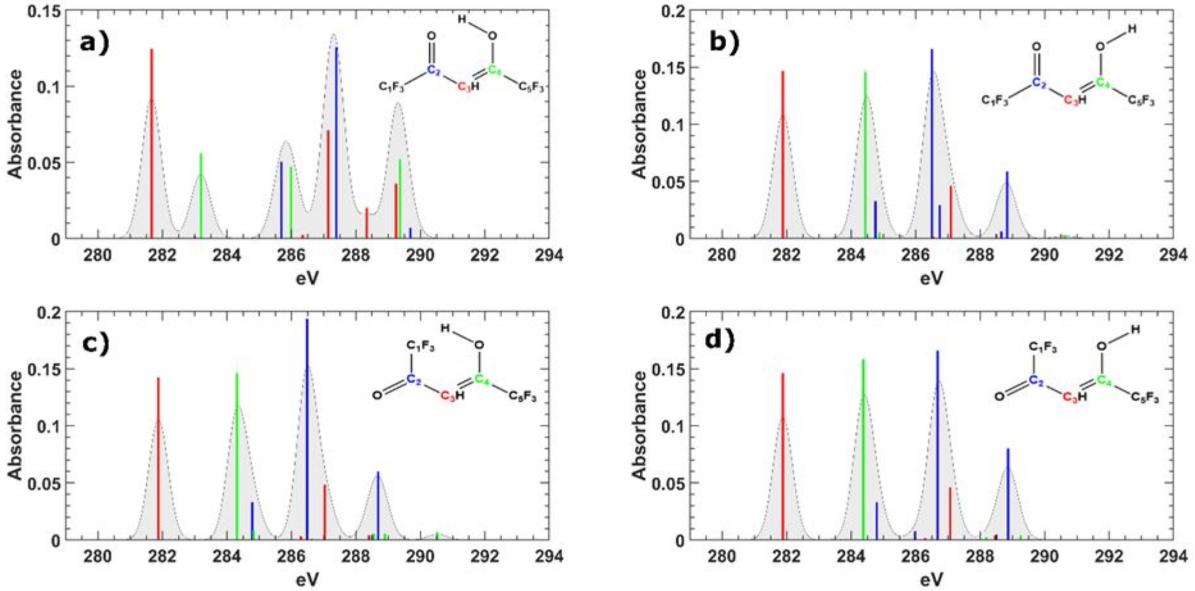


**Figure S9.** shows computed C K-edge OO-DFT spectra for four rotamers in the $T_1$ state, with a different basis set (aug-cc-pCVTZ for the core-hole site, aug-cc-pVDZ for all other atoms), focusing only on the central 3 carbon atoms. (a) corresponds to the CCC state, (b) corresponds to the CCT state, (c) corresponds to the TCC/TTC state and (d) corresponds to the TCT/TTT state.

The CCC state corresponds to a planar structure with the intramolecular hydrogen bond still intact. The other structures all correspond to a non-planar structure with no intramolecular hydrogen bond. Indeed, the $T_1$ state potentially allows free rotation about the $C_3$=$C_4$ bond, and thus there are fewer distinct rotamers possible than the ground state, since multiple $S_0$ state nonplanar rotamers collapse to the same $T_1$ structure upon geometry optimization. All the non-planar structures possess extremely similar calculated spectra. It was found that upon geometry optimization of the various rotamers that they are all within 2 kcal/mol of one another allowing for easy rotation between the isomers given the significant amount of energy gained upon relaxing from the $S_2$ state. It was seen that the experimental spectrum was best represented by a mixture of these rotamers rather than any single geometry.

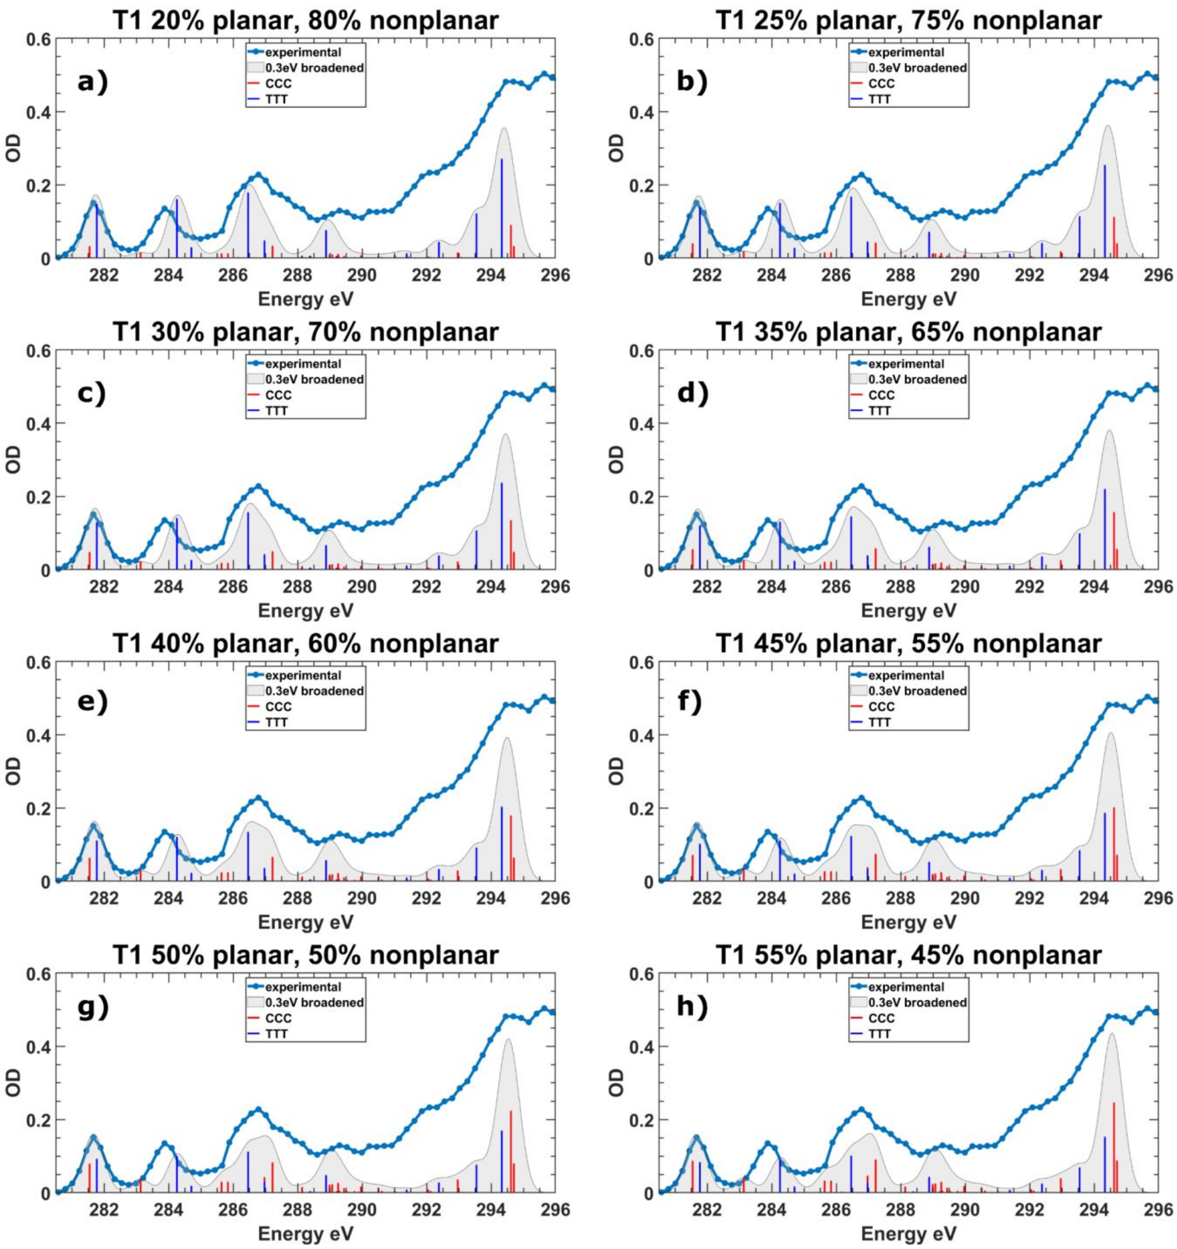


**Figure S10.** Relative fractions between the planar and nonplanar rotamers present in the $T_1$ electronic state. CCC represents the planar rotamers while TTT represents the nonplanar rotamers, the grey 0.3 eV broadened corresponds to the sum of the planar and nonplanar components.

## S9. Additional Kinetic Fits

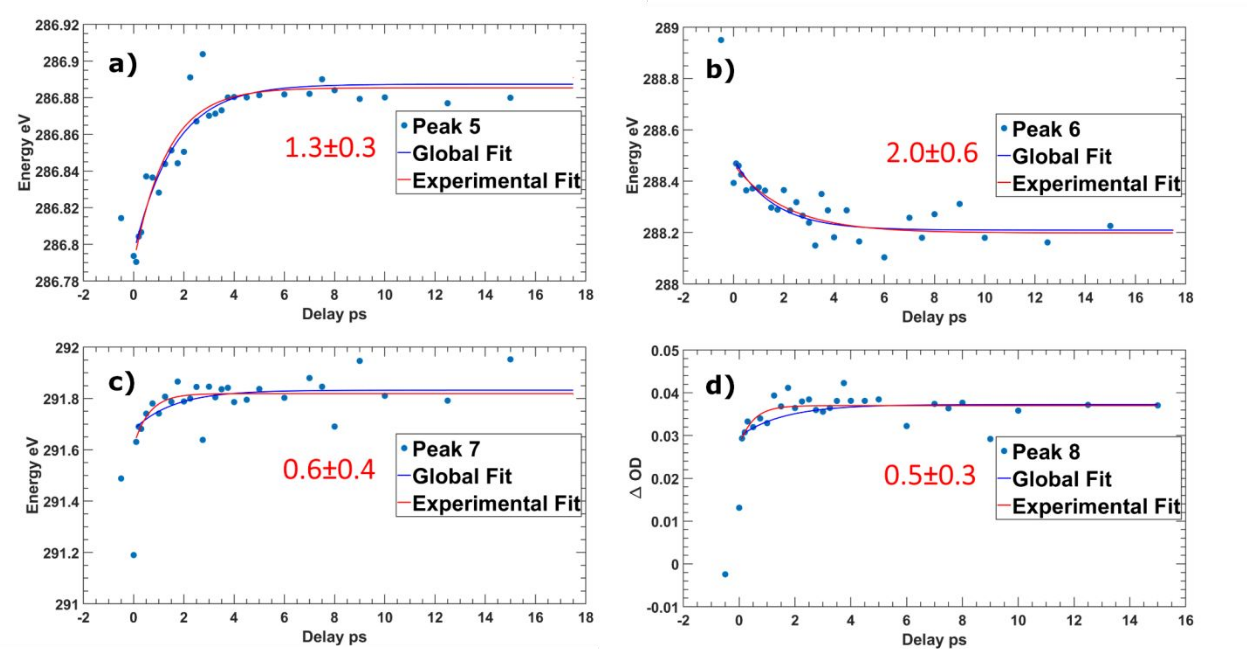


**Figure S11.** Energy shift of peaks 5, 6, 7 and the ΔOD of peak 8 are displayed as blue markers. Two fits are displayed: the blue corresponds to the global fit determined in the main paper and has a 1.6 ps exponential; the red fit represents the best individual fit for each peak where the value of each fit is displayed in units of picoseconds.

For peaks 5 and 6 there is a noticeable shift in energy corresponding to the intersystem crossing between $S_1 \rightarrow T_1$ states. This is based upon the similar rate constants displayed by peaks 1-4 which have been assigned to the intersystem crossing with the aid of theory in the main text. Based on the OO-DFT calculations, peaks 5 and 6 are predicted to primarily originate from $C_2$ and $C_4$.

However, the 1.6 ps exponential does not adequately fit peaks 7 and 8, which instead must be fit with an exponential on the order of 500 fs. This faster signal is only present at the high energy region of the spectrum where it is expected that excitations from the terminal $C_1$ and $C_5$ carbons will be predominant. Due to the relatively poor signal to noise ratio and limited experimental resolution, we are, at this time, unable to ascertain the exact mechanism producing this time dependence.

**References:**


1. A. R. Attar, A. Bhattacherjee, C. Pemmaraju, K. Schnorr, K. D. Closser, D. Prendergast and S. R. Leone, Science (New York,N.Y.), 2017, 356, 54—59.

2. Scutelnic, V.; Tsuru, S.; Papai, M.; Yang, Z.; Epshtein, M.; Xue, T.; Haugen, E.; Kobayashi, Y.; Krylov, A. I.; Møller, K. B.; Coriani, S.; Leone, S. R. X-ray transient absorption reveals the 1Au (nπ*) state of pyrazine in electronic relaxation. Nature Communications 2021,12, 5003.

3. O.-P. Sairanen, A. Kivimäki, E. Nõmmiste, H. Aksela and S. Aksela, Phys. Rev. A, 1996, 54, 2834–2839

4. M. Alagia, E. Bodo, P. Decleva, S. Falcinelli, A. Ponzi, R. Richter and S. Stranges, Phys. Chem. Chem. Phys., 2013, 15, 1310–1318

5. Nishijima, C.; Nakayama, H.; Kobayashi, T.; Yokota, K. PHOTOELECTRON SPECTRUM OF MALONALDEHYDE. Chemistry Letters 1975, 4, 5–8

6. R. J. Squibb, M. Sapunar, A. Ponzi, R. Richter, A. Kivimäki, O. Plekan, P. Finetti, N. Sisourat, V. Zhaunerchyk, T. Marchenko, L. Journel, R. Guillemin, R. Cucini, M. Coreno, C. Grazioli, M. Di Fraia, C. Callegari, K. C. Prince, P. Decleva, M. Simon, J. H. D. Eland, N. Došli´c, R. Feifel and M. N. Piancastelli, Nature Communications, 2018, 9, 63.

7. N. Kotsina, M. Candelaresi, L. Saalbach, M. M. Zawadzki, S. W. Crane, C. Sparling and D. Townsend, Phys. Chem. Chem. Phys., 2020, 22, 4647–4658

8. Muyskens, K. J.; Alsum, J. R.; Thielke, T. A.; Boer, J. L.; Heetderks, T. R.; Muyskens, M. A. Photochemistry of UV-Excited Trifluoroacetylacetone and Hexafluoroacetylacetone I: Infrared Spectra of Fluorinated Methylfuranones Formed by HF Photoelimination. The Journal of Physical Chemistry A 2012, 116, 12305–12313.
